# Supplementary material for: EviDial: When Correct Depression Predictions Lack Evidence
Source: arXiv:2610.27541 source file (2026-10-20)
Supplement: Supplementary file 1 [file appendix.tex]

% EviDial appendix: data and annotation first; historical results retain their references.
\section{Corpus, Label Provenance, and Windows}
\label{app:corpus}\label{app:accounting}

\begin{table}[htbp]
\centering\small
\caption{Processed EviDial sources. The 560 source-recorded identities include virtual or synthetic identities and must not be read as 560 clinical participants. Real-interview analyses use PDCH and EDAIC.}
\label{tab:corpus}
\begin{tabularx}{\linewidth}{@{}lXrl@{}}
\toprule
Source & Material & Transcripts / subjects & Label source \\
\midrule
PDCH & Real Chinese interviews & 99 / 72 & HAMD-17 \\
EDAIC & Real English interviews & 271 / 271 & PHQ-8 \\
TalkDep & LLM persona dialogues & 12 / 12 & Persona-derived \\
D4 & Trained simulation & 60 / 60 & Portrait risk \\
LingxiDiag & Disclosed synthetic & 52 / 52 & Four-class \\
MDD5K & Suspected synthetic & 51 / 51 & Unattributed \\
EATD & Real Chinese monologues & 42 / 42 & Severity labels \\
\bottomrule
\end{tabularx}
\end{table}

PDCH is a published multimodal interview dataset with HAMD-17 assessments \citep{pdch2025}. EDAIC belongs to the DAIC interview lineage \citep{gratch2014}; the cited corpus paper documents that lineage rather than independently verifying this release's label joins. PHQ-8 supplies depression items \citep{kroenke2009}; the PCL-C block is a separate comorbid-PTSD axis and is not used as a depression-item reference. LingxiDiag is described by its authors as synthetic \citep{lingxidiagbench2026}. EATD supplies real monologue material \citep{eatd2022}. TalkDep's persona-derived labels are silver rather than clinician ratings. Neither TalkDep nor MDD5K supports the label-dependent clinical analyses reported here.

\paragraph{Provenance checks.}
Version-controlled adapters extract instrument totals and items from publisher files. Thirty-seven PDCH totals are imputed by summing available items; they are not independent total-score measurements. The EDAIC join uses participant identifiers and has no upstream dialogue-session alignment check. Expansion labels were transcribed during the earlier panel run and subsequently checked against 205 original records, with no reported transcription mismatch. That verification establishes transcription fidelity, not clinical truth. Four EATD boundary cases at raw score 33 lack traceable tertile assignment and retain the raw score. Protocol blindness in the legacy run is supported by prompt and verdict audits; it is not a structural guarantee that the data pipeline could never expose labels.

\paragraph{Windows and item mappings.}
The revised task uses a one-week HAMD-17 window and a two-week PHQ-8 window. Legacy panel prompts used generic current-state framing, so they are not retrospectively treated as instrument-window-aligned annotations. BDI-II's usual two-week reference period does not establish the temporal provenance of LLM persona labels, which remain a separate tier. HAMD sleep combines three subitems, whereas PHQ-8 sleep is a single frequency item; their numerical scores are not pooled. HAMD concentration lacks a clean directly comparable item, and PHQ-8 has no suicidality item. A nine-dimension transcript schema does not imply nine observable scale labels per source.

\paragraph{Accounting.}\label{app:process}
The 2,935 planned protocol--transcript slots comprise 2,905 unique new verdict files and 30 traceable pilot reuses. A byte-identical duplicate is excluded from the file count. Each of 5,283 consensus cells has a five-vote basis. These are repeated protocol evaluations of the same material, not 26,415 independent clinical observations. The broader collection includes seven additional capability-training sources excluded from the evaluation claims.


\paragraph{Processed selection and source transformations.}
The 382-record core comprises 99 PDCH, 271 EDAIC, and 12 TalkDep transcripts. The extension is a selected 205-record set from D4, LingxiDiag, MDD5K, and EATD, not their full source inventories. Real interview data account for 370 transcripts from 343 people. The EDAIC text used in the processed collection is an LLM-reformatted representation; the current audit does not establish that all clinical meanings survive that transformation unchanged. The harmonized fields support provenance-aware joins, not psychometric equivalence between scales.

\paragraph{Annotation availability and duplicate checks.}
The core file has no populated L4 evidence layer. A separate 100-record proof-of-concept file has evidence fields on 96 records, totaling 538 dimension records. These added fields are model-generated. The five-protocol panel covers 5,283 unique cells with five votes each. Historical plurality counts are 2,378 positive, 869 negative, and 2,036 not-assessable, including 57 ties resolved by the legacy encounter-order rule. The atlas displays tied cells separately. A normalized exact-text comparison across the 587 processed records finds no duplicate groups; no near-duplicate or semantic-overlap guarantee follows.

\paragraph{Participant-split audit.}\label{app:splits}
The archived development and test manifests contain 24 and 120 cells. Development contains 24 distinct participants; the test manifest has 98 visit identifiers but 92 longitudinal participants. The generator copies the visit-level sample identifier into its subject field instead of grouping by the core longitudinal identifier. Three PDCH participants consequently occur in both manifests: participant 006 (development visit A, psychomotor; test visit B, fatigue), participant 014 (development visit B, concentration; test visit A, fatigue), and participant 019 (development visit A, appetite/weight; test visit B, guilt). This establishes participant overlap, not a quantified inflation in any score. The existing manifests and outputs remain archived. A valid independent evaluation requires all visits and dimensions of a participant to remain in one split, followed by versioned calibration and evaluation.

\section{Contract Details and Semantic Checks}
\label{app:measurement}

The frame contract separates interpretation from aggregation. A judge first resolves speaker, experiencer, dimension, temporal coverage, negation, and withdrawals; the aggregation function then derives $(U,K_r,A,Z)$. The executable checks operate on supplied frames. They do not verify that a model extracted the correct frames, that all decisive statements were found, or that a quoted substring supports the conclusion. Verbatim citation matching checks location only.

\paragraph{Sufficient negatives.}
The proposed convention requires a dimension-anchored denial covering the target window. Elicited and spontaneous denials are recorded separately. For suicidality, the annotation convention further restricts sufficient negatives to elicited denials; this is a conservative task choice, not a clinical rule that a denial establishes safety. The generic set aggregator does not itself enforce this evidence-class gate. A 30-cell re-adjudication of the legacy negative stratum retains 26 calls, with 27 denials judged dimension-anchored and four calls reclassified as absent or partial. This is agreement with a model reference, not validation by independent clinicians.

\paragraph{Semantic test suite.}
The suite covers other-person statements, unanswered clinician questions, retrospective versus current evidence, whole-utterance and cross-sentence negation, withdrawal, same-window conflict, repeated compatible statements, no evidence, relevant uncertainty, insufficient temporal coverage, granularity changes, and dimension anchoring. There are 13 base cases and two alternative readings. The current checker reproduces the expected $(U,K_r,A,Z)$ tuples on these supplied cases. An explicit positive statement and an explicit denial are tested through their permitted sets; the same positive range may be partial for an exact item score and sufficient for binary presence. These are local executable specifications, not an exhaustive test of natural-language reasoning.

\begin{table}[htbp]
\centering\small
\caption{Examples of the state mapping at binary presence granularity. The first column describes the \emph{resolved admissible} content, not an unverified keyword match.}
\label{tab:vars}
\begin{tabularx}{\linewidth}{@{}Xccl@{}}
\toprule
Content & $U$ & $K_r$ & State and polarity \\
\midrule
Explicit target-window affirmation & 1 & $\{1\}$ & Sufficient, positive \\
Explicit target-window denial & 1 & $\{0\}$ & Sufficient, negative \\
Patient addresses target but cannot say & 1 & $\{0,1\}$ & Partial, unresolved \\
No admissible patient statement & 0 & $\{0,1\}$ & Absent, unresolved \\
Unresolved opposing constraints & 1 & $\varnothing$ & Conflicting, unresolved \\
\bottomrule
\end{tabularx}
\end{table}

\paragraph{Temporal and semantic assumptions.}
The current implementation filters a pre-annotated coverage category; it does not independently derive interval relations from raw dates. It rejects narrower, wider, or unclear coverage. This is stricter than merely requiring temporal overlap and may exclude statements informative about binary presence. Its appropriateness must be assessed per instrument and question. Similarly, the granularity field does not validate a model's proposed allowed values automatically. Hand-specified cases demonstrate consistency of the set operations, not that the rules capture every clinically meaningful use of evidence.

\begin{table}[htbp]
\centering\small
\caption{\textbf{Binding determines what an answer is supported by.} Semantic operations illustrated by the sleep example and executable cases. The granularity row assumes all permitted item values are positive.}
\label{tab:binding}
\begin{tabularx}{\linewidth}{@{}>{\raggedright\arraybackslash}p{2.0cm}>{\raggedright\arraybackslash}X>{\raggedright\arraybackslash}p{4.3cm}@{}}
\toprule
Binding & Question resolved before scoring & Consequence under the contract \\
\midrule
Experiencer & Does the statement concern the patient? & A relative's symptom supplies no patient constraint. \\
Time & Does it cover the target assessment window? & An earlier episode does not resolve the current item. \\
Negation & Which assertion is denied? & A resolved denial permits $\{0\}$. \\
Withdrawal & Which earlier statement remains active? & Resolve withdrawal before intersecting constraints. \\
Granularity & Presence or exact item score? & $\{1,2\}$ is partial for score, sufficient after projection to presence. \\
\bottomrule
\end{tabularx}
\end{table}

\paragraph{Coverage-field boundary counterexample.}
An independent local audit finds that the implementation rejects several explicitly inadmissible coverage values but permits a frame whose coverage field is missing. With all other fields fixed, the counterexample yields sufficient-positive when coverage is omitted and absent when coverage is explicitly unclear. The frame schema also omits coverage from its required list. Passing the supplied semantic cases therefore does not establish complete input validation. This counterexample identifies a local boundary gap; it does not establish that every archived model output or reported score is affected. The manuscript revision reports this finding without changing the frozen experiment code or claiming corrected performance.

\section{Default Bound and Non-identifiability}
\label{app:theory}

\paragraph{Proposition (stratum-only accuracy bound).}
Fix a stratum $S$, let $q=P(Y=1\mid S)$, and let the predictor output 1 with probability $r$, independently of $Y$ conditional on $S$. Its expected accuracy is
\[
rq+(1-r)(1-q)=(1-q)+r(2q-1)\leq\max(q,1-q).
\]
The maximum is attained at $r=1$ if $q\geq1/2$ and $r=0$ otherwise. This includes deterministic predictors as endpoints and proves the bound for randomized stratum-only rules.

\paragraph{Decomposition and scope.}
For disjoint strata, define $\ell_S=\mathrm{Acc}_S-\max(q_S,1-q_S)$ and average over $S$ to obtain Equation~\ref{eq:default}. Lift is signed and may be negative. In the population, positive lift is incompatible with the stipulated conditional independence; it is not sufficient evidence of admissible text use because other information can correlate with $Y$. Nor is positive lift necessary for text use. A system can read and correctly interpret every explicit denial in a negative stratum while producing exactly the same outputs as a constant negative system. Estimated strata, sample priors, and sample accuracy add uncertainty beyond this elementary population statement.

\paragraph{Label-only non-identifiability.}
Consider two items with external label zero. One transcript contains an explicit admissible denial, while the other contains no admissible symptom evidence. A negative prediction is label-correct on both, but only the first is text-supported under the contract. Since the label score depends on $(\widehat Y,Y)$ and not on $(A,Z)$, its value cannot identify the support status. Even a full confusion matrix is insufficient: identical predictions can be generated by different decision procedures, and identical label correctness can accompany different support states. Reference labels and interventions answer different questions; neither can be reconstructed from accuracy alone.

\paragraph{Identical-text pairs.}\label{rem:balpair}
For two otherwise identical admissible model inputs with opposite hidden labels, a deterministic forced-binary predictor answers both the same way and is correct on exactly one. A randomized predictor with no access to the hidden pair member need not emit the same sampled answer twice, but has expected pair accuracy $1/2$. The statement requires identical visible metadata as well as identical text. The eight archived pairs check byte-identical evidence-removed renders; they should not be read as a general bound when identifiers or other side information leak the pair member. Their assertion-rate metric is distinct from this label-accuracy bound.

\section{Reference-Version and Granularity Audit}
\label{app:alignment}

The full contract and the constructed truth generator are separate implementations. Their labels must therefore be compared rather than presumed equivalent. The generator's family-I branch returns absent, while its rendered statement combines an earlier episode with an in-window inability to say. Under the revised relevance rule, the latter is an admissible inconclusive statement: $U=1$, $K_r=V_g$, and $A=\partl$. The difference affects a four-state status target even when both states map to abstention in binary decision scoring.

The 30-view comparison contains 15 sufficient presence references, 11 absent presence references, three conflicting presence references, and one partial item-score reference. All method prompts ask a presence question. The item-score case cannot be treated as a harmonized presence reference without re-evaluating its content at that granularity. The clean generator also records a generic current window, while the comparison runner asks about the past week. These mismatches do not justify silently replacing archived labels; they require a new, versioned, contract-aligned reference and sensitivity scoring of the frozen outputs.

The proposed label-support indicator in Section~\ref{sec:model} uses entailment. Some archived support fields instead test membership of $Y$ in a permitted set, and absent states are serialized with an empty set rather than the full candidate domain plus $U=0$. No numerical $B$ prevalence claim is based on treating these representations as interchangeable. Formal definitions, reference serialization, and scoring must be versioned together before a confirmatory evaluation.

\section{Human Annotation Assets and Reference Reliability}
\label{app:human}

\subsection{Existing double annotations on real PDCH interviews}

\paragraph{Provenance and linkage.}
The project supplies two original human annotation returns, each containing 99 completed records, alongside blinded packets and an annotation guide. The authors report that these annotations had not been used in the earlier EviDial analyses. This is a statement about annotation use, not unseen transcripts: all 99 interviews already belong to the core and were used in the legacy model panel. Matching packet records to the core verifies speaker roles, exact turn text, and turn order for every interview. The linked cohort contains 72 participants, with 27 contributing two visits. The 198 completed returns are therefore 99 paired interview judgments, not 198 participants or an independent test cohort.

\paragraph{Original protocol and analysis scope.}
Annotators first assess whether enough patient narrative is available, then label evidence domain, ideation, behavior, plan, intent, means access, temporal status, evidence status, confidence, and retrospective review priority. They select original turns as supporting spans. The guide prohibits access to the other annotator's decisions, weak labels, and model outputs. We describe this as the documented blinding procedure; return files alone cannot verify compliance or professional qualifications. Reported comparisons use the two initial returns, preserving disagreement. Neither model-simulated adjudication nor a majority vote supplies a final human reference. No completed task-aligned human adjudication was found in the audited assets.

\paragraph{Agreement computation.}
Section~\ref{sec:annotation} states the participant-cluster procedure, and Table~\ref{tab:human} reports all six fields, including intent and means access. Each field uses all 99 paired records and unweighted Cohen's $\kappa$. All bootstrap kappas were defined. Intervals are unadjusted for multiple fields and conditional on this source and annotator pair; they do not establish population reliability or a statistically significant ordering of fields.

\paragraph{Disagreement anatomy.}
The 50 plan-absence/unknown pairs all have annotator A choosing \texttt{absent} and B choosing \texttt{unknown}; these account for 50/73 plan disagreements (68.5\%). Another 20 pairs oppose absent and present. For means access, A chooses \texttt{none\_mentioned} and B chooses \texttt{unknown} on 35 interviews. Historical versus current/recent disagreements total 26: A chooses current/recent and B historical on 21, and the reverse occurs on five. Ideation differs on 39 interviews, including 26 active/passive pairs. Both raters choose active or passive on 76 interviews and none on ten; nine pairs oppose an ideation category and none, and four involve ambiguity. These post-hoc summaries describe label choices and possible review targets, without diagnosing their semantic cause or identifying which rater is correct.

\paragraph{Evidence boundaries.}
The raters agree on explicit-span evidence in 78 interviews and on explicit denial in ten. Eight pairs oppose span and denial, and three oppose span and insufficient evidence. A located quotation does not by itself establish the experiencer, target window, or answer granularity. Current/recent labels do not certify past-week coverage, and an ideation label of none does not by itself establish a supported negative. The old plan value \texttt{absent} describes a component, whereas EviDial's \absent\ describes absence of admissible evidence. Consequently, these fields are not automatically recoded into $(A,Z)$ or used to score the archived model comparisons. Their reuse for that purpose requires full-context, target-aligned review and adjudication, including disputed cases.

\subsection{Auxiliary expert annotations on synthetic narratives}

\paragraph{Unit and raw results.}
A separate export contains 100 completed single-expert ratings and 200 blank rows. Only the 100 completed ratings are analyzed. An earlier 52-rating export is a subset, not an additional sample. The 100 synthetic narratives correspond to 95 source anchors, including five original/cleaned pairs; anchors are not independent clinical participants. These narratives are auxiliary to the 587-transcript collection. The original final-state field contains 95 passive-ideation and five high-concern-component judgments. The original sufficiency field contains 72 \texttt{insufficient\_evidence} and 28 \texttt{sufficient\_negative\_evidence} values. Of the 72 insufficient records, 68 have a passive-ideation classification and four a high-concern-component classification. The legacy negative-evidence wording must not be read as absence of ideation: all 28 such records also have one of these two positive-content categories.

\paragraph{Raw judgments and retrospective interpretation.}
The expert supplied a subsequent rubric distinguishing classifiability of ideation from completeness of the wider safety assessment: missing positive follow-up does not erase an ideation judgment. A separately stored projection labels 75 records as incomplete positive follow-up, 23 as complete without means assessment, and two as complete. This 75 is a derived rubric count, not the original 72 or 75 newly collected expert judgments. Three current-behavior projections use rubric-defined inference rather than a direct denial. We preserve these distinctions and use the asset to motivate target-specific granularity, without importing its branching rules into EviDial's evidence contract.

\paragraph{Quality and generalization.}
Section~\ref{sec:human-findings} reports the usability counts. The 42 questionnaire-wording flags comprise 27 mild and 15 obvious cases; the 11 consistency flags comprise four minor issues and seven major contradictions. These are quality flags on this selected synthetic asset, not prevalence estimates for EviDial. One expert cannot establish between-rater agreement, and an all-positive-content sample cannot validate negative-answer or abstention performance. Separate 180-item legacy assets have unresolved annotator-provenance documentation in the audited records; expansion templates and agent-simulated candidates are also excluded from the reported human results.

\subsection{Model reference repeatability and remaining human validation}

\paragraph{Within-model samples.}
The 46-view repeatability analysis uses two views for each of 23 targets. The three GPT-mini samples include the original API response and additional samples at temperatures .5 and .8. They therefore probe sensitivity to sampling settings as well as repeatability; they are not three identical-temperature replications. Sufficiency is unanimous for 35 views and split for 11; pairwise kappas are .734, .493, and .547. One view receives three different statuses. A tie-breaking procedure can still produce a decision, but such a decision must be reported as a tie-break rather than a majority.

\paragraph{Between-family pilot.}
The 12 shared cells give raw sufficiency agreement $2/12$ and Cohen's $\kappa=0.047619$. The margins are 11 sufficient and one partial for GPT-mini, versus one sufficient, seven partial, and four absent for Gemini-lite. The expected chance agreement under these margins is $18/144=.125$, so $(2/12-.125)/(1-.125)=.047619$. The source record states that the run stopped after disagreement became apparent. This outcome-dependent stopping and the single-source, legacy-positive sample limit interpretation. The observed disagreement motivates further reference validation; it neither estimates a corpus-wide rate nor identifies which judge is correct. An earlier 11-cell summary is superseded by the 12-cell record.

\paragraph{Separate planned EviDial annotation.}
The earlier 82-cell EviDial-specific package remains unfilled in its support, polarity, and quotation fields; it is distinct from the completed 24-cell pilot analyzed below. It contains 44 core cells and 38 comparison cells, plus 16 planned repeat judgments. Thus it has 82 distinct cells and 98 planned ratings if completed. The core allocation includes 30 positive external labels. Stratum quotas are purposive; within-stratum selection is randomized in the frozen plan. The annotator package hides external labels, legacy assignments, and system outputs, with a private join after reference freezing. A later model-disagreement priority list is a separate proposed selection rule; using it would change the target population and must not be described as outcome-blind sampling.

One qualified annotator can establish task feasibility, ambiguity patterns, and within-rater repeatability after a washout. That design cannot estimate between-rater agreement or produce an adjudicated multi-clinician reference. The cost estimate of approximately 26 hours for the core stage uses a placeholder reading speed and requires a timed pilot. The quoted $\pm23$-percentage-point precision is conditional on an assumed rate and effective denominator, not a general precision guarantee for all 44 core cells. No annotation result, prevalence estimate, or clinical performance measure is reported from the prepared package.

\paragraph{Required estimands.}
Unsupported correct predictions can occur when either label is zero or one. The primary analysis should distinguish (i) the fraction of all eligible predictions that both match $Y$ and lack sufficient text support, and (ii) the fraction of label hits lacking support. Positive-label oversampling is a design choice, not a logical prerequisite for this phenomenon. Unsettled human ratings should remain a separate uncertainty category, with prespecified sensitivity bounds. Population estimates require sampling weights, a stated eligible population, and clustering where several cells come from one participant.

\input{pilot_annotations}
\input{scoped_candidate}

\section{Stratification and Mismatch Cases}
\label{app:audit}\label{app:strata-details}

\begin{table}[htbp]
\centering\small
\caption{Three partitions must be kept distinct. ``Other'' pools partial, absent, and conflicting states. Majority default is $\max(q,1-q)$, not necessarily the positive-label rate $q$.}
\begin{tabular}{@{}llrrrr@{}}
\toprule
Partition & Stratum & $n$ & $q$ & Default & Accuracy \\
\midrule
Legacy, initial & Positive & 15 & .867 & .867 & .933 \\
 & Negative & 15 & .267 & .733 & .733 \\
 & Not-assessable & 15 & .467 & .533 & .533 \\
\midrule
Legacy, GPT extension & Positive & 30 & .633 & .633 & .667 \\
 & Negative & 30 & .233 & .767 & .767 \\
 & Not-assessable & 29 & .483 & .517 & .517 \\
\midrule
Frozen revised, GPT & Sufficient-positive & 11 & .818 & .818 & .818 \\
 & Sufficient-negative & 12 & .583 & .583 & .583 \\
 & Other & 22 & .364 & .636 & .591 \\
\bottomrule
\end{tabular}
\end{table}

The initial legacy strata use a three-valued judgement, not the later four-state sufficiency contract. All 15 initial not-assessable cells and 14 of the 15 negative cells are EDAIC; eight of the positive cells are PDCH. The GPT extension targets 30 per stratum but has 29 usable not-assessable cells. Enlarged-sample priors differ from the initial priors and are not interchangeable with them.

\paragraph{Re-adjudication.}
An 18-cell grid samples six cells from each legacy stratum across three sources. Two re-readers agree on status and polarity in 16/18 cells. Only three of six legacy positive calls remain sufficient-positive; two change to negative and one to partial. The not-assessable group contains four agreed absences, one agreed sufficient-positive, and one disagreement. This demonstrates differences between procedures in a small selected grid. It does not establish that the legacy panel over-calls half of all positive cells, because there is no independent validated reference and each stratum has only six observations.

In the frozen 45-cell re-adjudication by Gemini-lite and Qwen-plus, joint agreement is 28/45. Of the 15 legacy positive cells, nine remain sufficient-positive and six become sufficient-negative. Of the 15 negative cells, one becomes positive, five stay negative, and nine become other. The 15 not-assessable cells split 1/1/13. The resulting group sizes are 11/12/22. The original system scores .909/.750/.636 against defaults .818/.583/.636; a mixed-prompt sensitivity partition makes the positive default .909 and removes that positive lift. These are reference-sensitivity checks rather than independent confirmations.

\begin{table}[htbp]
\centering\small
\caption{Frozen-partition benchmark audit. Accuracies and lifts differ across families; all reported bootstrap intervals for lift include zero. This supports uncertainty about above-default performance, not equality to the default.}
\label{tab:audit}
\begin{tabular}{@{}llrrrr@{}}
\toprule
Model & Stratum & $n$ & Acc. & Default & Lift \\
\midrule
GPT-mini & Sufficient-positive & 11 & .818 & .818 & .000 \\
 & Sufficient-negative & 12 & .583 & .583 & .000 \\
 & Other & 22 & .591 & .636 & $-.045$ \\
\midrule
Gemini-lite & Sufficient-positive & 11 & 1.000 & .818 & $+.182$ \\
 & Sufficient-negative & 12 & .667 & .583 & $+.083$ \\
 & Other & 22 & .727 & .636 & $+.091$ \\
\midrule
Qwen-plus & Sufficient-positive & 11 & .909 & .818 & $+.091$ \\
 & Sufficient-negative & 12 & .583 & .583 & .000 \\
 & Other & 22 & .682 & .636 & $+.045$ \\
\bottomrule
\end{tabular}
\end{table}

\paragraph{Eight inspected discrepancies.}\label{app:cases}
Four cases have panel-positive judgements against scale zeros. PDCH\_004A/anhedonia contains the patient's explicit statement of loss of interest at turn 91, while HAMD item 7 is zero. This is a candidate discrepancy, not an adjudicated label error: item 7 covers work and activities more broadly, and time anchoring and complete context need review. PDCH\_008A/suicidality combines a past self-harm impulse with denial of current suicidal intent; treating the former as current is a panel error. EDAIC\_330/concentration maps forgetfulness to attention, and EDAIC\_333/concentration compares a presence judgement with a frequency item. These two cases concern mapping and granularity rather than a demonstrated inconsistency in the patient's state.

The four opposite-direction cases are EDAIC\_677, EDAIC\_450, and EDAIC\_617 for anhedonia, and EDAIC\_410 for depressed mood. Panel-negative judgements cite activities or positive affect while the items score one or two. Such counter-evidence does not necessarily deny symptoms over two weeks. Candidate explanations include insufficient negative evidence, a narrower reading of current state, interview--questionnaire differences, and participant-level linkage. The eight cases are purposively inspected examples; they do not define a validated taxonomy or a denominator for prevalence.

\paragraph{A majority can miss time binding.}
The PDCH\_043A example is presented in Section~\ref{sec:binding}. It is a purposive illustration of shared temporal error, with concentration excluded from the eight scored dimensions; it does not estimate how often majority voting introduces such an error.

\section{Constructed Failure Checks}
\label{app:constructed}

The development templates cross six archetypes with eight dimensions, producing 48 scenarios and four views per scenario. The held-out construction has seven families across eight dimensions: new positive and negative expressions plus five additional combinations. Removing evidence, matched material, or paraphrased filler produces 224 views from 56 scenarios. There are 72 sufficient-negative views under the archived rules. The frozen seed is 20260908. The numerical tolerances are status accuracy $\geq.98$, joint sufficient-negative correctness $\geq.90$, unsupported assertions on absent views $\leq.05$, supported-answer rate $\geq.95$, conditional polarity accuracy $\geq.95$, and balanced-pair assertion rate $\leq.05$.

\begin{table}[htbp]
\centering\small
\caption{Programmed systems scored against archived clean-template labels. Every non-oracle system fails at least one criterion. Columns A, N, U, V, P, and B are the six criteria defined below. ``--'' means no eligible conditional-polarity denominator.}
\label{tab:failure}
\begin{tabular}{@{}lrrrrrr@{}}
\toprule
System & A $\uparrow$ & N $\uparrow$ & U $\downarrow$ & V $\uparrow$ & P $\uparrow$ & B $\downarrow$ \\
\midrule
Oracle & 1.000 & 1.000 & .000 & 1.000 & 1.000 & .000 \\
Always insufficient & .357 & .000 & .000 & .000 & -- & .000 \\
Keyword positive & .411 & .000 & .113 & .031 & .143 & .000 \\
Question as evidence & .357 & .000 & .000 & .000 & -- & .000 \\
Ignore subject & .411 & .000 & .113 & .031 & .143 & .000 \\
Ignore time & .411 & .000 & .113 & .031 & .143 & .000 \\
Length only & .393 & .000 & .500 & .125 & .250 & .500 \\
Source cue & .429 & .500 & 1.000 & .500 & .500 & 1.000 \\
Mimic judge & .411 & .000 & .113 & .031 & .143 & .000 \\
Always positive & .429 & .000 & 1.000 & .250 & .250 & 1.000 \\
\bottomrule
\end{tabular}
\end{table}

A is status accuracy; N requires both sufficient status and negative direction among reference sufficient-negative views. U measures definite assertions on reference absent views. V measures definite, direction-correct answers on sufficient views. P conditions on both reference and system declaring sufficient. B measures sufficient claims on the 16 members of eight balanced pairs, all absent under the archived labels. A system is detected if any criterion is violated. The table demonstrates detection of the specified systems; several have identical output profiles, and no inference about unseen failure classes follows.

\paragraph{Metric correction.}
The original negative metric ignored polarity. Always-positive therefore obtained 72/72 sufficient-status recall on negative items. Joint scoring reduces its negative correctness to 0/72. The old statistic is retained only as a sufficiency-recall diagnostic; its threshold is no longer interpreted as negative-judgement validity. Reusing a numerical tolerance after correcting the target metric is transparent, but does not make the corrected metric prospectively preregistered.

\paragraph{Regeneration and judge checks.}
The original filler included a diet exchange that could supply negative appetite evidence. Regeneration replaces it with neutral weather text and retains the scenario count, 72 negative views, and eight identical pairs. ``Clean'' refers to this repair alone. The 24-view clean judge subset yields qwen-plus 23/24 status accuracy, 6/6 sufficient negatives, and 14/14 absent views; Gemini-lite yields 19/24, 5/6, and 12/14. Earlier pre-regeneration checks included single-run status accuracy of approximately .83--.92 for four additional models, and five GPT-mini runs ranging .50--.96 with a majority-vote result .958. These are different sets and procedures; they do not constitute a common six-family validation sample.

\section{Method Implementations and Calibration}
\label{app:calibration}

All three model families receive the same transcript and target within a comparison: gpt-5-mini, gemini-2.5-flash-lite, and qwen-plus. Direct answering permits abstention; evidence-first additionally asks for binding checks and a quoted statement. The sufficient-context adaptation uses the published one-shot autorater prompt \citep{sufficientcontext2025}, a forced-binary answer with confidence, and a locally fitted logistic decision rule. Structured prompting asks the model to extract frames, derive the candidate set, and report status and polarity in the same call. The scorer maps non-sufficient status to abstention. This is a prompted implementation; the experiment does not replace model-reported aggregation with a separately verified deterministic inference step.

\begin{table}[htbp]
\centering\small
\caption{Actual configured completion limits per unit and model. Limits are not measured token consumption. The final decision space is shared; cost is not matched.}
\label{tab:budgets}
\begin{tabularx}{\linewidth}{@{}>{\raggedright\arraybackslash}X>{\raggedright\arraybackslash}p{1.2cm}>{\raggedright\arraybackslash}p{2.2cm}>{\raggedright\arraybackslash}p{2.3cm}@{}}
\toprule
Method & Calls & Constructed & Real-cell run \\
\midrule
Direct + abstention & 1 & 1,200 & 1,200 \\
Evidence-first & 1 & 2,500 & 1,600 \\
Sufficient-context & 2 & 1,200 + 2,500 & 1,200 + 3,000 \\
Structured frames & 1 & 4,000 & 6,000 \\
Confidence-only & 0 extra & Reuses answer stage & Not calibrated \\
\bottomrule
\end{tabularx}
\end{table}

The constructed comparison prompts specify presence over the past week. The 30 shared views and three models produce 90 model--view records and 450 stage calls. The confidence-only scorer reuses the forced-binary answer stage's confidence and answer, not the direct-with-abstention output. This differs from the earlier prose specification. It is therefore a confidence-only ablation of that answer stage, not a clean estimate of the incremental contribution of confidence to the direct method.

\input{method_components}

\paragraph{Fitted decision rule.}
The sufficient-context head computes $p=\sigma(\beta_0+\beta_1s+\beta_2c)$, where $s$ is binary autorater sufficiency and $c$ is self-rated confidence. It commits if $p\geq\eta$ and otherwise abstains. The search grid is $\beta_0\in[-6,2]$, $\beta_1\in[-4,4]$, and $\beta_2\in[-2,6]$, all at steps of .5, with $\eta=.05,.10,\ldots,.95$. Fitting to $J$ on 90 model--view rows gives $\beta=[-6,1.5,2]$, $\eta=.05$, and in-sample $J=.789$. An alternative direction-correctness target gives $[-5.5,1,6]$, $\eta=.50$. These parameter changes are target-dependent, not a sign reversal of the sufficiency coefficient; both reported sufficiency coefficients are positive. Several optima touch the grid boundary.

\paragraph{Cross-validation leakage.}
The archived five-fold routine shuffles 90 model--view rows with seed 20260911. It does not group the three models' records for a view. Reconstructing that split finds another record of the same view in training for 87 of the 90 evaluation rows. Thus the reported $.756$ is a row-level cross-validation diagnostic with shared-view leakage. It must not be described as scoring each unseen view with a head that has never encountered that view. A valid replacement should keep all models, views, and related instances from the same base scenario together, with fitting and evaluation decisions frozen before examining the new result. No corrected cross-validation performance is asserted in this revision.

Confidence-only uses threshold .90 selected in-sample against direction correctness, whereas the sufficient-context head's primary target is $J$. Moreover, a direction-correctness target on non-sufficient cells depends on an arbitrary treatment of unresolved polarity and is not equivalent to grounded correctness. These design asymmetries are additional reasons not to infer a method ranking from the fitted rows.

\paragraph{Real-cell run and technical failures.}
The 120-cell comparison contains 1,799 of 1,800 recorded stage calls. One GPT evidence-first cell repeatedly fails parsing and is not imputed. The autorater has ten unparsed Gemini outputs and five unparsed Qwen outputs, despite completed transport calls. Its sufficient counts are 79/120 for GPT, 37/120 for Gemini, and 46/120 for Qwen. Parsing failures must be distinguished from valid insufficiency decisions. Structured output initially truncated under a smaller budget and was rerun with a larger limit; it has 360 recorded outputs after repair. The final structured decisions are positive/negative/insufficient counts 21/42/57 for GPT, 21/95/4 for Gemini, and 30/61/29 for Qwen. These are observable behaviours and do not require a correctness reference.

\section{Within-Case Intervention Details}
\label{app:intervention}

Of 28 enrolled subjects (24 targets and four controls), one target lacks locatable evidence spans; 27 subjects yield 216 views-by-task units per model arm. The primary deletion contrast uses 23 targets. A verbatim check finds no retained quoted spans in evidence-removed views, with evidence-removed/matched-removed character ratios .90--1.04. This does not exclude paraphrased evidence, changes in discourse coherence, or content accidentally deleted by the control.

\begin{table}[htbp]
\centering\small
\caption{Deletion-response estimates. $W/L/T$ are wins, losses, and ties for matched-minus-evidence definiteness; sign tests exclude ties. Original rows use a merged model-arm record. Majority-vote rows use three GPT-mini samples.}
\label{tab:tau-full}
\begin{tabular}{@{}llrrrr@{}}
\toprule
Analysis & Source & $n$ & $W/L/T$ & $\tau$ & $p$ \\
\midrule
Original evidence & All & 23 & 9/3/11 & $+.261$ & .146 \\
 & EDAIC & 16 & 8/1/7 & $+.438$ & .039 \\
 & PDCH & 7 & 1/2/4 & $-.143$ & 1.000 \\
Original label & All & 23 & 9/2/12 & $+.304$ & .065 \\
 & EDAIC & 16 & 6/2/8 & $+.250$ & .289 \\
 & PDCH & 7 & 3/0/4 & $+.429$ & .250 \\
\midrule
Majority-vote evidence & All & 23 & 8/1/14 & $+.304$ & .039 \\
 & EDAIC & 16 & 8/0/8 & $+.500$ & .008 \\
 & PDCH & 7 & 0/1/6 & $-.143$ & 1.000 \\
\bottomrule
\end{tabular}
\end{table}

\paragraph{Arm composition and inference.}
The complete cross-family arm contains all 216 units; 171 also have an original-family record. Frozen source priority selects original-family verdict, repair, inline record, then cross-family API response. Among the 46 target-by-task pairs, 18 mix families and 28 do not (24 original-family pairs and four GPT pairs). The count of 23 mixed pairs in an older report includes the four controls and has a denominator of 54, not 46. Mixing families confounds the contrast with model identity. All-GPT re-scoring gives evidence $\tau=.304$ ($p=.065$), EDAIC .563 ($p=.004$), PDCH $-.286$, and zero label-task response. These are separate estimates from the majority-vote rows.

The original six tests are the two tasks crossed with all/EDAIC/PDCH. None of the original single-call results passes Bonferroni $\alpha=.05/6$. In the later majority-vote check, EDAIC's exact $p=.0078125$ passes that numerical threshold but the pooled $p=.0390625$ does not. This limited correction does not account for all later analyses or convert the follow-up into a preregistered confirmatory study.

\paragraph{Threshold and contamination sensitivity.}
The label-confidence threshold .70 was chosen with knowledge of earlier exploratory analyses. At .5/.6/.7/.8, label $\tau$ is .00/.04/.30/.22, with $W/L/T=0/0/23$, $1/0/22$, $9/2/12$, and $9/4/10$. PDCH\_008A is included in the 23-target table despite a diagnosed panel error in evidence location. Its contrasts are ties. Removing it leaves the same nonzero contrasts and sign-test results, but changes the denominator to 22 and the estimates to .318 for labels and .273 for evidence. Thus exclusion leaves the qualitative conclusion unchanged, not the numerical effect.

\paragraph{Controls and source differences.}
Matched deletion changes evidence sufficiency from .739 to .565; its non-inertness means the contrast compares two potentially meaningful perturbations. It is neither an isolated causal effect nor a proven lower bound. A residue audit finds higher remaining target-related density in EDAIC (.23) than PDCH (.11), although EDAIC has the larger deletion response. This does not support the proposed redundancy explanation. Language, length, dimension mix, and temporal scope remain confounded with source.

Four normal controls receive 20/20 sufficient-negative votes on a later five-judge re-reading. Two global-affect controls would become absent under the stricter elicited-only convention. This is a small diagnostic repair, not held-out validation. An earlier unarchived analysis reported $\tau=.13$ and could not be reproduced under the explored priorities and thresholds; it is withdrawn and does not contribute to the present estimates.

\section{Distractor Design and Condition Integrity}
\label{app:mechanism}

The experiment contains 64 base scenarios: four distractor types, two target polarities, and eight dimensions. Each scenario has four evidence-by-distractor views. All views have 13 turns, but adding distractor content changes character length. Evidence-first and structured outputs are evaluated alongside the forced-binary answer stage used by sufficient-context. The latter is not the final calibrated selective method.

\begin{table}[htbp]
\centering\small
\caption{Full family-specific distractor contrasts. Each transition reports distractor absent to present. All rows use the same 64 base scenarios; model rows are not independent scenario replications.}
\begin{tabular}{@{}llccc@{}}
\toprule
Method & Model & Unsupported commitment & Supported error & $\Delta$ \\
\midrule
Evidence-first & GPT & $.453\to.359$ & $.000\to.016$ & $-.109$ \\
 & Gemini & $.250\to.281$ & $.000\to.000$ & $+.031$ \\
 & Qwen & $.000\to.203$ & $.000\to.000$ & $+.203$ \\
\midrule
Answer stage & GPT & $1.000\to1.000$ & $.000\to.000$ & $.000$ \\
 & Gemini & $1.000\to1.000$ & $.000\to.000$ & $.000$ \\
 & Qwen & $1.000\to1.000$ & $.000\to.000$ & $.000$ \\
\midrule
Structured & GPT & $.578\to.406$ & $.000\to.031$ & $-.203$ \\
 & Gemini & $.984\to.844$ & $.094\to.094$ & $-.141$ \\
 & Qwen & $.000\to.203$ & $.016\to.000$ & $+.219$ \\
\bottomrule
\end{tabular}
\end{table}

The reported 95\% intervals use 2,000 bootstrap draws clustered by the 64 base scenarios, keeping repeated views and model-family responses together. The pooled evidence-first contrast is $.042$ with interval $[-.052,.135]$; structured is $-.042$ with $[-.120,.042]$. These intervals do not establish the absence of an effect. Family-specific point estimates motivate replication and explicit heterogeneity analysis, rather than an untested claim that population effects necessarily have opposite signs.

\paragraph{Saturated baseline.}
The forced-binary answer stage never abstains in 768 evaluated views. Unsupported commitment is 1 in both evidence-absent arms and the reported supported error is zero in both evidence-present arms. Its contrast and bootstrap interval are therefore exactly zero by the observed saturation, not evidence of robustness to distractors. Calibrating the full selective method is necessary before comparing its abstention response with the other methods.

\paragraph{Withdrawal repair.}
An earlier withdrawal render included a replacement assertion that described the current week as fine. That replacement was admissible negative evidence, so treating the view as unsupported produced incorrect scoring. The renderer was changed to withdrawal without replacement, the truth table was derived from the stated contract, and the 768 affected calls were rerun. An earlier significant contrast was withdrawn. Twelve evidence-first calls that initially failed parsing were recovered with a larger budget. The final analysis reports 3,072 stage calls, which includes the autorater stage and should not be confused with 3,072 independent scenarios.

No single distractor category has the highest structured commitment across all three models. The archived per-type summaries pool the two distractor arms, so they describe category-associated behaviour and are not, by themselves, isolated causal effects of adding that category. Claims about a universal strongest distractor are unsupported.

\section{Historical Risk--Coverage and Safety Diagnostics}
\label{app:riskcov}

These results use the pre-regeneration constructed unit set and its earlier references. They are retained for traceability and hypothesis generation; they are excluded from the main method claim because the repaired text and later contract were not used to produce them.

\begin{table}[htbp]
\centering\small
\caption{Historical matched-coverage operating points. Risk is error among answered units under the earlier reference. The Google and Anthropic variants differ from models in the current 30-view comparison. No statistical superiority is inferred.}
\begin{tabular}{@{}lrrrr@{}}
\toprule
Model & $n$ & Coverage & Structured risk & Direct risk \\
\midrule
gpt-5-mini & 60 & .600 & .306 & .417 \\
gemini-2.5-flash & 30 & .433 & .385 & .538 \\
claude-haiku-4-5 & 30 & .133 & .500 & .500 \\
\bottomrule
\end{tabular}
\end{table}

The Anthropic point rests on four answered units. The GPT set includes a 30-unit extension. Equal coverage does not imply that two systems answer the same cases, and a favourable operating point does not establish dominance across the curve. Earlier reports of improved abstention against a forced-binary baseline also conflate a protocol difference with provision of an abstention option; the direct-with-abstention comparison addresses that specific confound.

A historical ten-unit suicidality probe contains seven evidence-removed absent views and three full partial/conflicting views. Forced-binary systems produce no positive answers on the seven absent views; direct and evidence-first produce positive answers on two of the three full views, while structured abstains on all three and on nine of ten views overall. These small, reference-specific counts do not estimate clinical harm or safety, and do not justify deployment claims.

\section{Artifact Map and Reference Versions}
\label{app:artefacts}

The source workspace separates the paper from experimental artifacts. The main anchors are: \texttt{T01\_contract} for the frame contract, semantic cases, and metric specification; \texttt{e0\_holdout} for generated views, template truth, calibration, and label-stratum audits; \texttt{e2\_pilot/analysis} for deletion responses and repeated judgements; \texttt{T02\_reference\_harness} for the surrogate pilot and unfilled human package; \texttt{T05\_runner} for the 120-cell and 30-view comparisons; and \texttt{T08\_mechanism} for factorial distractor responses. The T-prefixed directories reside under the dated revision directory. The original paper supplement indexes corresponding copies; it does not contain the entire harmonized clinical corpus. Historical directory names are retained to preserve traceability after the EviDial rename.

For the 30-view comparison, the authoritative scored record is \texttt{constructed\_scores.json}, paired with \texttt{constructed\_out\_clean} and \texttt{views\_clean}. The older output directory and superseded score file are not the main result. Likewise, \texttt{surrogate\_scores.json} is a model-annotation result, not a human reference. Directories marked as synthetic self-tests or quarantined analysis are excluded from every scientific claim.

The archived scores remain attached to the reference version and fitting procedure that produced them. Reference alignment and grouped calibration require separately versioned outputs before a confirmatory method comparison can be made. The earlier prepared 82-cell package is unfilled; the existing human component returns address an earlier task, and the separate completed 24-cell pilot is reported in Appendix~\ref{app:pilot-panel}. Semantic checks and arithmetic consistency establish local properties of the measurement pipeline; they do not resolve these scientific validation gaps.

\paragraph{Manuscript version and independent recount.}
EviDial names the dataset and benchmark design in this revision. Earlier MEGA and DEPTH labels remain in archived project paths and historical planning documents; they do not denote additional datasets. This manuscript reorders the presentation around source construction, annotation quality, benchmark tasks, and findings, while retaining frozen model results and adding secondary analysis of existing human annotations. A separate read-only recount checks collection sizes, panel votes and plurality ties, populated annotation fields, participant overlap, and the missing-coverage counterexample. Those checks establish the stated artifact properties, not independent clinical reference validity. The paper source bundle includes the text, bibliography, unmodified conference style, and figures; experimental records remain separate, under their applicable source restrictions.


\paragraph{Human-audit records.}
The source inventory, transcript-linkage checks, and analysis script are stored under \texttt{evidial\_v2/reviews/}, in the folder \texttt{aaai\_human\_assets\_20260916}. The script \texttt{analyze\_support.py} uses the project's participant-cluster reliability routine. The original source returns reside in the separate \texttt{aaai\_p1\_p2} project. Source SHA-256 hashes, six-field confusion matrices, and expert aggregate counts are included in \texttt{human\_audit\_summary.json} in the paper source package. Original clinical text and participant mappings remain outside that package. No annotation is overwritten, no new human rating is solicited, and no model API is called for this secondary analysis.
