# Supplementary material for: EviDial: When Correct Depression Predictions Lack Evidence
Source: arXiv:2610.27541 source file (2026-10-20)
Supplement: Supplementary file 2 [file appendix.tex]

% Appendix: detailed technical content moved from the main text.

\section{Dataset Details}
\label{app:dataset}

The four-state evidence contract (Equation~\ref{eq:states}) assigns states through the following admissibility rules. An evidence frame is admissible if: (a) the speaker is the patient or a direct reporter of the patient's state; (b) the temporal scope falls within the declared assessment window; (c) the evidence granularity matches the dimension's operational definition. Withdrawal resolution precedes state assignment: if a patient first endorses and then explicitly denies a symptom within the same window, the denial governs. The 18-item semantic adjudication register covers: temporal scope interpretation (R01--R03), speaker attribution rules (R04--R05), evidence granularity boundaries (R06--R08), denial admissibility (X1--X4), and six additional disambiguation items (N01--N06). All 18 items were frozen before judging.

The estimand family classifies each prediction against the independent reference:
\begin{itemize}
\item \textbf{C} (correct): label matches reference and evidence supports the label.
\item \textbf{U} (unsupported): label matches but reference shows insufficient evidence.
\item \textbf{D} (direction-wrong): label matches but reference supports opposite polarity.
\item \textbf{R} (unresolved): label matches but reference state is unresolved.
\item \textbf{N}: all planned predictions (the denominator).
\end{itemize}
The primary estimand is $(U{+}D)/(N{-}R)$ with sensitivity bounds $[(U{+}D)/N,\;(U{+}D{+}R)/N]$, always reported with the unresolved share $R/C$.

\section{Metrology: Mathematical Details}
\label{app:metrology}

\subsection{Generalizability Theory Decomposition}

The crossed person $\times$ unit-within-person $\times$ protocol design decomposes vote variance as:
\[
y_{puc} = \mu + \alpha_p + \beta_{u:p} + \gamma_c + (\alpha\gamma)_{pc} + \epsilon_{puc}
\]
where $p$ indexes participants, $u$ indexes cells within participants, and $c$ indexes protocols. Protocol is treated as fixed (five specific protocols, not a random sample from a universe of protocols); all other facets are random. Variance components are estimated by equating observed mean squares to their expectations. The D-study reliability coefficient is:
\[
E\rho^2(n) = \frac{\sigma^2_{\beta}}{\sigma^2_{\beta} + \sigma^2_{\epsilon}/n}
\]
where $\sigma^2_\beta$ is the cell-within-participant variance (the ``true'' differentiation among cells) and $\sigma^2_\epsilon$ is the residual. The effective judge count is computed from the eigenvalue spectrum of the $5\times 5$ vote-covariance matrix: $n_{\mathrm{eff}} = (\sum_i \lambda_i)^2 / \sum_i \lambda_i^2$.

\subsection{Many-Facet Rasch Model}

For each submeasure ($A$: assessable; $B$: direction$\mid$assessable), the conditional maximum-likelihood model is:
\[
\log \frac{P(y_{uc}=1 \mid \theta_u, \beta_c)}{P(y_{uc}=0 \mid \theta_u, \beta_c)} = \theta_u - \beta_c
\]
where $\theta_u$ is the cell parameter and $\beta_c$ is the protocol severity. The homogeneity test is a conditional likelihood-ratio test of $H_0: \beta_1 = \cdots = \beta_5$. The bias-corrected consensus uses empirical Bayes posteriors from the fitted model, with continuous posteriors eliminating the tie-break artifact of discrete plurality voting.

\subsection{Random-Effects Latent-Class Model}

The model posits $K$ latent classes with a shared random intercept:
\[
P(\mathbf{y}_u \mid b_u) = \sum_{k=1}^{K} \pi_k(x_u) \prod_{c=1}^{C} P(y_{uc} \mid k, b_u)
\]
where $b_u \sim N(0, \sigma^2)$ is the shared random effect, $\pi_k(x_u)$ are covariate-dependent mixing proportions, and the emission probabilities $P(y_{uc} \mid k, b_u)$ depend on the class and the random effect. Integration over $b_u$ is by Gauss--Hermite quadrature on a fixed grid. The covariate extension parameterizes $\log(\pi_k / \pi_K) = x_u' \gamma_k$, where $x_u$ includes source indicators and dimension-group indicators.

\section{Perturbation Anchor Design}
\label{app:anchors}

Eight perturbation classes, each with construction preconditions:
\begin{enumerate}
\item \textbf{Evidence deletion}: remove all admissible evidence for a dimension. Precondition: no residual synonymous evidence after deletion.
\item \textbf{Withdrawal}: insert explicit retraction of previously endorsed symptom. Precondition: endorsement exists in base view.
\item \textbf{Explicit-denial insertion}: insert clear denial statement. Precondition: no contradicting evidence in target window.
\item \textbf{Distractor insertion}: insert irrelevant but plausible clinical content. Precondition: distractor is topically related but dimensionally orthogonal.
\item \textbf{Out-of-window symptom}: insert symptom statements outside the assessment window (the PDCH\_043A probe). Precondition: in-window evidence remains intact.
\item \textbf{Half-support}: engineer partial evidence (yields \partl{}). Precondition: evidence is genuinely ambiguous.
\item \textbf{Same-window contradiction}: insert contradicting evidence within window (yields \confl{}). Precondition: both sides of contradiction are individually valid.
\item \textbf{Window-incomplete denial}: insert denial that does not cover the full assessment window. Precondition: residual endorsement remains.
\end{enumerate}
Generator-family exclusivity ensures injected text comes from a model family belonging to neither the judging panel nor the evaluated systems.

\section{Calibration Gate History}
\label{app:calibration}

\begin{table}[!htbp]
\centering\small
\caption{\textbf{Instrument calibration history.} Three bounded gate rounds plus two model eliminations.}
\label{tab:calibration}
\begin{tabular}{@{}llrr@{}}
\toprule
Round & Action & Merged validity & Notes \\
\midrule
Pre-calibration & Initial assessment & 37.3\% & Five judge candidates \\
Gate 1 & Prompt refinement & 58.1\% & Format compliance focus \\
Mini-gate 1 & DeepSeek gen-1 test & 21.9\% & \textbf{Eliminated} \\
Gate 2 & Schema alignment & 74.2\% & Language-split detected \\
Mini-gate 2 & DeepSeek gen-2 test & 18.8\% & \textbf{Eliminated} \\
Gate 3 & Language stratification (A3) & 87.0\% & Final panel composition \\
\bottomrule
\end{tabular}
\end{table}

The language-stratified panel (Amendment~A3): English layer (2{,}168 EDAIC cells) judged by gemini-2.5-flash and qwen3.8-max; Chinese layer (576 PDCH cells) by qwen3.8-max and claude-sonnet-4-6. Strong-judge calibration subsample: 796 cells. Second-family control: 100 cells.

\section{Construct Validity Evidence Map}
\label{app:validity}

\begin{table}[!htbp]
\centering\small
\caption{\textbf{Construct-validity evidence (Messick's six facets).}}
\label{tab:validitymap}
\begin{tabularx}{\linewidth}{@{}l>{\raggedright\arraybackslash}X>{\raggedright\arraybackslash}X@{}}
\toprule
Facet & Evidence in EviDial & Status \\
\midrule
Content & 18-item adjudication register; four-state contract grammar & Frozen \\
Substantive & Four states derive from evidence-support structure, not label convenience & Frozen \\
Structural & MFRM decomposition; protocol severity; bias-corrected consensus & Frozen \\
Generalizability & G-theory decomposition; cross-family panel with mutual-exclusion & Frozen / design \\
External & Anchor Se/Sp; validation sets; terminal audit & Partial / pending \\
Consequential & Interpretation boundary; claim ladder; misuse boundary & Frozen \\
\bottomrule
\end{tabularx}
\end{table}
